# Supplementary material for: Theory for the conditioned spectral density of non-invariant random matrices
Source: arXiv:1803.03314 ancillary file (2018-08-13)
Supplement: Supplementary file 1 [file SupMatvFinal.pdf]

# Supplemental Information: theory for the conditioned spectral density of non-invariant random matrices

Isaac Pérez Castillo
*Department of Quantum Physics and Photonics, Institute of Physics,*
*UNAM, P.O. Box 20-364, 01000 Mexico City, Mexico and*
*London Mathematical Laboratory, 14 Buckingham Street, London WC2N 6DF, United Kingdom*

Fernando L. Metz
*Institute of Physics, Federal University of Rio Grande do Sul, 91501-970 Porto Alegre, Brazil*
*Physics Department, Federal University of Santa Maria, 97105-900 Santa Maria, Brazil and*
*London Mathematical Laboratory, 14 Buckingham Street, London WC2N 6DF, United Kingdom*

## I. THE CONDITIONED SPECTRAL DENSITY FROM THE REPLICA METHOD

In this section we explain the essence of our theoretical approach, namely, how the replica method of disordered systems can be used to rewrite the conditioned spectral density in terms of a saddle-point integral, which is readily evaluated in the limit $N \to \infty$. Let us consider an ensemble of $N \times N$ symmetric random matrices $\boldsymbol{M}$ with real entries and eigenvalues $\lambda_1, \dots \lambda_N$. Since we make no additional assumptions regarding the random matrix ensemble, the approach presented below is valid for a broad class of random matrices, including those that break rotational invariance. The observable of interest here is the eigenvalue distribution constrained to have $kN$ $(0 \leq k \leq 1)$ eigenvalues smaller than $x$. This quantity is defined as follows

$$\rho_x(\lambda|k) = \lim_{N\to\infty} \frac{\left\langle \frac{1}{N}\sum_{i=1}^N \delta(\lambda-\lambda_i)\delta\left[kN - \mathcal{I}_N(x)\right]\right\rangle}{\left\langle \delta\left[kN-\mathcal{I}_N(x)\right]\right\rangle}, \tag{1}$$

where $\langle \dots \rangle$ is the ensemble average with the distribution of $\boldsymbol{M}$, while $\mathcal{I}_N(x)$ denotes the number of eigenvalues smaller than $x \in \mathbb{R}$, also known as the *index* of the random matrix $\boldsymbol{M}$. The threshold $x$ and the fraction $k$ of eigenvalues smaller than $x$ are parameters that can be independently controlled. By representing the Dirac delta constraining the index $\mathcal{I}_N(x)$ as an integral, we obtain

$$\rho_x(\lambda|k) = \lim_{N\to\infty} \frac{\int_{-i\infty}^{i\infty} dy\, e^{ykN} \left\langle \frac{1}{N}\sum_{i=1}^N \delta(\lambda-\lambda_i) e^{-y\mathcal{I}_N(x)}\right\rangle}{\int_{-i\infty}^{i\infty} dy\, e^{ykN}\left\langle e^{-y\mathcal{I}_N(x)}\right\rangle}. \tag{2}$$

One has to express the arguments in the numerator and denominator of eq. (2) as functions of $\boldsymbol{M}$, such that the ensemble averages can be, in principle, calculated. This is achieved by using the following identity for the index [6,31]

$$\mathcal{I}_N(x) = \sum_{i=1}^N \Theta\left(x-\lambda_i\right) = \lim_{\epsilon\to 0^+}\frac{1}{2\pi i}\left[\sum_{i=1}^N \mathrm{Log}(\lambda_i + i\epsilon - x) - \sum_{i=1}^N \mathrm{Log}(\lambda_i - i\epsilon - x)\right], \tag{3}$$

which is based on a relation between the Heaviside function $\Theta(\dots)$ and the discontinuity of the principal complex logarithm $\mathrm{Log}(\dots)$ along the negative imaginary axis. Let us then introduce the following multidimensional Fresnel integral

$$Z(x_\epsilon) = \int d\boldsymbol{y} \exp\left[-\frac{i}{2}\boldsymbol{y}^T\left(x_\epsilon \mathbb{I} - \boldsymbol{M}\right)\boldsymbol{y}\right] = (2\pi)^{\frac{N}{2}} \exp\left[-\frac{1}{2}\sum_{i=1}^N \mathrm{Log}(\lambda_i + i\epsilon - x) + i\frac{N\pi}{4}\right], \quad x_\epsilon = x - i\epsilon\,, \tag{4}$$

with $\boldsymbol{y}^T = (y_1, \dots, y_N)$ and $\mathbb{I}$ is the $N \times N$ identity matrix. Then Eq. (3) is rewritten as

$$\mathcal{I}_N(x) = \lim_{\epsilon\to 0^+}\frac{1}{\pi i}\left[\mathrm{Log}\overline{Z(x_\epsilon)} - \mathrm{Log}Z(x_\epsilon) + \frac{N\pi i}{2}\right], \tag{5}$$

where $\overline{(\dots)}$ stands for complex conjugation. Notice that since the exponential and complex logarithm are not injective functions in the complex plane, many standard properties of these functions defined over $\mathbb{R}$ do not apply when working in $\mathbb{C}$. We have clearly ignore this when going from Eq. (3) to Eq. (5). However, this non-rigorous step is crucial to apply the replica technique and calculate the ensemble average (we refer to the appendix of [33] for a careful discussion of this issue). This procedure has

been recently employed to compute the cumulant generating function of the index, leading to compelling results for the typical and atypical index fluctuations of random graphs [31,32] and sparse Wishart random matrices [33]. Substituting the above equation back in Eq. (2), we obtain

$$\rho_x(\lambda|k) = \lim_{N\to\infty}\lim_{\epsilon\to 0^+} \frac{\int_{-i\infty}^{i\infty} dy\, e^{yN\left(k-\frac{1}{2}\right)} \left\langle \frac{1}{N}\sum_{i=1}^N \delta(\lambda-\lambda_i) \left[\overline{Z(x_\epsilon)}\right]^{-\frac{y}{\pi i}} \left[Z(x_\epsilon)\right]^{\frac{y}{\pi i}} \right\rangle}{\int_{-i\infty}^{i\infty} dy\, e^{yN\left(k-\frac{1}{2}\right)} \left\langle \left[\overline{Z(x_\epsilon)}\right]^{-\frac{y}{\pi i}} \left[Z(x_\epsilon)\right]^{\frac{y}{\pi i}} \right\rangle}. \tag{6}$$

We still have to express the Dirac delta $\delta(\lambda-\lambda_i)$ in terms of $\boldsymbol{M}$. This is achieved by noticing that

$$\sum_{i=1}^N \delta(\lambda-\lambda_i) = -\frac{1}{\pi}\lim_{\eta\to 0^+} \mathrm{Im}\left[\sum_{i=1}^N \frac{1}{\lambda_i-\lambda+i\eta}\right] = -\frac{2}{\pi}\lim_{\eta\to 0^+} \mathrm{Im}\left[\frac{\partial}{\partial\lambda_\eta}\mathrm{Log}Z(\lambda_\eta)\right], \quad \lambda_\eta = \lambda - i\eta. \tag{7}$$

By inserting eq. (7) in eq. (6), we get the following expression

$$\rho_x(\lambda|k) = -\frac{2}{\pi}\lim_{N\to\infty}\lim_{\epsilon\to 0^+}\lim_{\eta\to 0^+}\frac{1}{N}\mathrm{Im}\left[\frac{\frac{\partial}{\partial\lambda_\eta}\int dy\, e^{yN\left(k-\frac{1}{2}\right)} \left\langle \mathrm{Log}[Z(\lambda_\eta)] \left[\overline{Z(x_\epsilon)}\right]^{-\frac{y}{\pi i}} \left[Z(x_\epsilon)\right]^{\frac{y}{\pi i}} \right\rangle}{\int dy\, e^{yN\left(k-\frac{1}{2}\right)} \left\langle \left[\overline{Z(x_\epsilon)}\right]^{-\frac{y}{\pi i}} \left[Z(x_\epsilon)\right]^{\frac{y}{\pi i}} \right\rangle}\right]. \tag{8}$$

Equation (8) suggests that $\rho_x(\lambda|k)$ follows from the solution of a saddle-point integral. Actually, notice that an expression of the sort $\left\langle \mathcal{O}\left[\overline{Z(x_\epsilon)}\right]^{-\frac{y}{\pi i}} \left[Z(x_\epsilon)\right]^{\frac{y}{\pi i}} \right\rangle$, similarly as Eq. (8), for some generic quantity $\mathcal{O}$, can be understood solely based on probabilistic grounds. To see this, let us first introduce $N\Delta\epsilon = \frac{i}{\pi}\mathrm{Log}\left(\frac{Z(x_\epsilon)}{\overline{Z(x_\epsilon)}}\right)$. Then the previous average takes the following form $\left\langle \mathcal{O}e^{-yN\Delta\epsilon}\right\rangle$ which, in this new light, involves a Boltzmann-type measure with a fictitious inverse temperature $y$. The role of this temperature is precisely to bias the ensemble such that atypical events become typical. Moreover, we should expect that $\left\langle \mathcal{O}e^{-yN\Delta\epsilon}\right\rangle = \mathcal{O}(y)e^{-yN\mathcal{G}(y)}$, so the goal is to find a way to obtain mathematical expressions for $\mathcal{O}(y)$ and $\mathcal{G}(y)$. However, we still have an issue, as the numerator in Eq. (8) involves the coupling between $Z(x_\epsilon)$ and $\mathrm{Log}Z(\lambda_\eta)$ through the ensemble average. Applying the standard replica method of disordered systems [30], solely in the function $\mathrm{Log}Z(\lambda_\eta)$, one can derive the expression

$$\left\langle \mathrm{Log}[Z(\lambda_\eta)] \left[\overline{Z(x_\epsilon)}\right]^{-\frac{y}{\pi i}} \left[Z(x_\epsilon)\right]^{\frac{y}{\pi i}} \right\rangle = Q_0^{(N)}(y,x_\epsilon)\lim_{n\to 0}\frac{1}{n}\mathrm{Log}\left(\frac{Q_n^{(N)}(y,\lambda_\eta,x_\epsilon)}{Q_0^{(N)}(y,x_\epsilon)}\right), \tag{9}$$

where we have defined

$$Q_n^{(N)}(y,\lambda_\eta,x_\epsilon) = \left\langle \left[\overline{Z(x_\epsilon)}\right]^{\frac{iy}{\pi}} \left[Z(x_\epsilon)\right]^{-\frac{iy}{\pi}} \left[Z(\lambda_\eta)\right]^n \right\rangle. \tag{10}$$

Notice that a similar quantity has been introduced in the study of ensembles of loopy random graphs [38]. The final step consists in plugging eq. (9) in eq. (8), which enables to recast $\rho_x(\lambda|k)$ as follows

$$\rho_x(\lambda|k) = -\frac{2}{\pi}\lim_{N\to\infty}\lim_{\epsilon\to 0^+}\lim_{\eta\to 0^+}\lim_{n\to 0}\frac{1}{Nn}\mathrm{Im}\left[\frac{\partial}{\partial\lambda_\eta}\frac{\int dy\, e^{N\left[yk-\mathcal{F}^{(N)}(y,x_\epsilon)\right]}\mathrm{Log}\left[Q_n^{(N)}(y,x_\epsilon,\lambda_\eta)\right]}{\int dy\, e^{N\left[yk-\mathcal{F}^{(N)}(y,x_\epsilon)\right]}}\right], \tag{11}$$

with

$$\mathcal{F}^{(N)}(y,x_\epsilon) = \frac{y}{2} - \frac{1}{N}\ln Q_0^{(N)}(y,x_\epsilon). \tag{12}$$

The integral over $y$ in eq. (11) is promptly evaluated, in the limit $N\to\infty$, through the saddle-point method, yielding a formal expression for the conditioned spectral density

$$\rho_x(\lambda|k) = -\frac{2}{\pi}\lim_{\eta\to 0^+}\lim_{\epsilon\to 0^+}\lim_{n\to 0}\frac{1}{n}\mathrm{Im}\left[\frac{\partial}{\partial\lambda_\eta}\lim_{N\to\infty}\frac{1}{N}\mathrm{Log}\left[Q_n^{(N)}(y_\star,x_\epsilon,\lambda_\eta)\right]\right], \tag{13}$$

with $y_\star$ obtained from the stationary condition

$$k = \frac{\partial\mathcal{F}(y,x_\epsilon)}{\partial y}\Big|_{y=y_\star}, \quad \mathcal{F}(y,x_\epsilon) = \lim_{N\to\infty}\mathcal{F}^{(N)}(y,x_\epsilon). \tag{14}$$

Equation (13) is one of the main outcomes of our theoretical approach: this equation shows that the calculation of $\rho_x(\lambda|k)$ is reduced to the computation of the $N \to \infty$ limit of $Q_n^{(N)}(y_\star, x_\epsilon, \lambda_\eta)$, evaluated at the extrema of $\mathcal{F}(y, x_\epsilon)$ with respect to $y$. We stress that our theory for the conditioned spectral density does not rely on any specific properties of the random matrix ensemble, such as rotationally invariance [1], and it can be applied to a broad class of random matrices. One may follow once more the common strategy of the replica approach and obtain the analytic form of $Q_n^{(N)}$, for fixed integer $n > 0$, from the limiting procedure

$$Q_n^{(N)}(y_\star, x_\epsilon, \lambda_\eta) = \lim_{n_\pm \to \pm \frac{iy_\star}{\pi}} \left\langle \left[\overline{Z(x_\epsilon)}\right]^{n_+} \left[Z(x_\epsilon)\right]^{n_-} \left[Z(\lambda_\eta)\right]^n \right\rangle. \tag{15}$$

At first, one considers $n_\pm$ to be positive integers and computes the ensemble average on the right hand side. Once this has been done and the leading contribution for $N \to \infty$ has been extracted, the original function $Q_n^{(N)}$ of the continuous variable $y_\star$ is reconstructed through the replica limit $n_\pm \to \pm \frac{iy_\star}{\pi}$. In order to pursue this plan, one has to specify the random matrix ensemble, since the right hand side of eq. (15) is given in terms of the ensemble average of an intricate function. In this work, we have computed $Q_n^{(N)}(y_\star, x_\epsilon, \lambda_\eta)$ and obtained $\rho_x(\lambda|k)$ for the ensemble of the adjacency matrix of Erdös-Rényi (ER) random graphs and for sparse Wishart random matrices. The final equations determining $\rho_x(\lambda|k)$ for ER random graphs are shown in the main text of the paper, while the analogous equations for sparse Wishart random matrices are presented in the next section. We will not discuss here all technical details involved in the replica derivation of $Q_n^{(N)}(y_\star, x_\epsilon, \lambda_\eta)$, since this follows similar steps as those discussed thoroughly in [32,33], where the cumulant generating function of the index has been calculated for the same random matrix ensembles as discussed here.

## II. ANALYTIC EXPRESSION FOR THE CONDITIONED SPECTRAL DENSITY OF SPARSE WISHART MATRICES

The ensemble of sparse Wishart random matrices is defined in the main text. The only difference here is that the equations below are also valid in the more general situation where the nonzero elements of $\boldsymbol{\xi}$ are identically and independently drawn from an arbitrary distribution $P_\xi(\xi)$. In the main text, we have discussed explicit results for the simplest choice $P_\xi(\xi) = \delta(\xi - 1)$. The calculation of the function $Q_n^{(N)}(y_\star, x_\epsilon, \lambda_\eta)$ for such ensemble follows a similar derivation as the one explained carefully in [33]. Thus, here we simply report the final equations determining the conditioned spectral density. The function $\rho_x(\lambda|k)$ follows from

$$\rho_x(\lambda|k) = \frac{1}{\pi} \lim_{\eta \to 0^+} \lim_{\epsilon \to 0^+} \int_{-\infty}^{\infty} d\Gamma w_{y_\star}(\Gamma) \text{Im}\Gamma, \quad d\Gamma = d\text{Re}\Gamma \, d\text{Im}\Gamma \,, \tag{16}$$

with

$$w_{y_\star}(\Gamma) = \int_{-\infty}^{\infty} d\Omega \, w_{y_\star}(\Omega, \Gamma), \quad d\Omega = d\text{Re}\Omega \, d\text{Im}\Omega \,. \tag{17}$$

The distribution $w_{y_\star}(\Gamma)$ is obtained from the solution of the following self-consistency system of equations involving the distributions $w_{y_\star}(\Omega, \Gamma)$, $w_{y_\star}^{(1)}(\omega, \gamma)$, and $w_{y_\star}^{(2)}(\Sigma, \sigma)$

$$w_{y_\star}(\Omega, \Gamma) = \frac{1}{\mathcal{N}} \sum_{\ell=0}^{\infty} \mathcal{A}^\ell \int \left[\prod_{s=1}^{\ell} d\omega_s \, d\gamma_s \, w_{y_\star}^{(1)}(\omega_s, \gamma_s)\right] \exp\left[-\frac{iy_\star}{2\pi} \text{Log}\left(\frac{\sum_{s=1}^{\ell} \omega_s - x_\epsilon}{\sum_{s=1}^{\ell} \overline{\omega}_s - \overline{x_\epsilon}}\right) + \frac{iy_\star}{2\pi} \sum_{s=1}^{\ell} \text{Log}\left(\frac{\omega_s}{\overline{\omega}_s}\right)\right]$$
$$\times \, \delta\left[\Omega - \frac{1}{\left(\sum_{s=1}^{\ell} \omega_s - x_\epsilon\right)}\right] \delta\left[\Gamma - \frac{1}{\left(\sum_{s=1}^{\ell} \gamma_s - \lambda_\eta\right)}\right], \tag{18}$$

$$w_{y_\star}^{(1)}(\omega, \gamma) = \int d\Sigma \, d\sigma \, w_{y_\star}^{(2)}(\Sigma, \sigma) \left\langle \delta\left[\omega - \frac{\xi^2}{c\,(\Sigma + 1)}\right] \delta\left[\gamma + \frac{\xi^2}{c\,(\sigma + 1)}\right]\right\rangle_\xi, \tag{19}$$

$$w_{y_\star}^{(2)}(\Sigma, \sigma) = \sum_{\ell=0}^{\infty} \frac{c^\ell e^{-c}}{\ell!} \int \left[\prod_{k=1}^{\ell} d\Omega_k \, d\Gamma_k \, w_{y_\star}(\Omega_k, \Gamma_k)\right] \left\langle \delta\left(\Sigma - \frac{1}{c} \sum_{k=1}^{\ell} \xi_k^2 \Omega_k\right) \delta\left(\sigma - \frac{1}{c} \sum_{k=1}^{\ell} \xi_k^2 \Gamma_k\right)\right\rangle_{\xi_1, \dots, \xi_\ell}, \tag{20}$$

with

$$\mathcal{A} = \alpha c \left\{\int d\Sigma \, d\sigma \, w_{y_\star}^{(2)}(\Sigma, \sigma) \exp\left[\frac{iy_\star}{2\pi} \text{Log}\left(\frac{1 + \overline{\Sigma}}{1 + \Sigma}\right)\right]\right\}^{-1}. \tag{21}$$

The symbol $\langle \dots \rangle_\xi$ represents the average over the random variable $\xi$ with the distribution $P_\xi(\xi)$, while the normalization factor $\mathcal{N}$ ensures that $\int_{-\infty}^{\infty} d\Omega\, d\Gamma\, w_{y_\star}(\Omega, \Gamma) = 1$. As we mentioned in the main text, $y_\star$ is found from the stationary condition $k = \frac{\partial \mathcal{F}(y,x_\epsilon)}{\partial y}\Big|_{y=y_\star}$, where the explicit form for the cumulant generating function $\mathcal{F}(y, x_\epsilon)$ for Wishart random matrices is presented in [33].

## III. ESTIMATING $y_\star$ FROM THE WEIGHTED POPULATION DYNAMICS ALGORITHM

In order to calculate the conditioned spectral density, we need to determine the value of $y_\star$ corresponding to a fixed fraction $k$ of eigenvalues smaller than $x$. In fact, the self-consistency equations for the distributions in the case of ER random graphs (see the main text) and sparse Wishart random matrices (see eqs. (18-20)) depend on $y_\star$, which is obtained from $k = \frac{\partial \mathcal{F}(y,x_\epsilon)}{\partial y}\Big|_{y=y_\star}$. In order to find $y_\star$ for a certain $k$, we use the Newton's method. Essentially, the value $y = y_\star$ corresponds to the zero of the function $f(y) = k - \kappa_1(y)$, in which $\kappa_1(y)$ is defined according to

$$\kappa_1(y) = \frac{\partial \mathcal{F}(y, x_\epsilon)}{\partial y}. \tag{22}$$

Notice that $\kappa_1(y)$ is actually the first cumulant of $\mathcal{I}_N(x)$ in the conditioned ensemble, so we are looking for the value $y_\star$ that will indeed give that $k = \kappa_1(y_\star)$. In the Newton's method, one finds a sequence of approximations for $y_\star$ by iterating the following equation

$$y^{(t+1)} = y^{(t)} - \frac{\left[\kappa_1(y^{(t)}) - k\right]}{\kappa_2(y^{(t)})}, \quad t = 0, 1, \dots, \tag{23}$$

where $y^{(0)}$ is an initial guess for $y_\star$. Here $\kappa_2(y) = -\frac{\partial^2 \mathcal{F}(y,x_\epsilon)}{\partial y^2}$, which corresponds to the second cumulant of $\mathcal{I}_N(x)$ in the conditioned ensemble. Obviously, $\kappa_1(y)$ and $\kappa_2(y)$ yield, respectively, the first and second cumulants of the index in the unconstrained ensemble when calculated at $y = 0$. Since we have the analytic forms of $\mathcal{F}(y, x_\epsilon)$ for ER random graphs (see the main text) and sparse Wishart random matrices [33], simple expressions for $\kappa_1(y)$ and $\kappa_2(y)$ are derived. We point out that, luckily, such derivation requires only explicit derivatives of $\mathcal{F}(y, x_\epsilon)$ with respect to $y$, but not implicit ones.

Numerically, the approach is simple: given a certain $y^{(t)}$, one uses the weighted population dynamics, thoroughly discussed in [32], to obtain an estimate for the functions $\kappa_1(y^{(t)})$ and $\kappa_2(y^{(t)})$, which subsequently provide the next value $y^{(t+1)}$ through eq. (23). The iteration is stopped after $y^{(t)}$ converges to its asymptotic value $y_\star$. In figure 1 we illustrate this method by applying it to the ensemble of ER random graphs with $c = 5$ and $P_J(J) = (1//\sqrt{2\pi/c})e^{-cJ^2/2}$ (see the main text). During the iteration process, the population size $\mathcal{N}$ in the weighted population dynamics algorithm is increased linearly from $\mathcal{N} = 10^6$ to $\mathcal{N} = 10^7$ as a function of $t$. Moreover, due to the stochastic nature of the population dynamics algorithm, results are averaged over 100 independent realizations. In Figure 1 we present the sequence of approximations for $\kappa_1^{(t)} \equiv \kappa_1(y^{(t)})$ (left figure) and $y^{(t)}$ (middle figure). Besides that, the right panel of Figure 1 exhibits the standard deviation $\delta\kappa_1^{(t)}$ of $\kappa_1^{(t)}$ among different runs of the population dynamics method, with the purpose to give an idea of the accuracy of our numerical calculations. Notice how in the right plot of Figure 1 $\delta\kappa_1^{(t)}$ approaches asymptotically to a small but non-zero value. This is consistent with the population size we have used, if we naïvely assume that the population dynamics algorithm displays fluctuations among different runs that behave as $O(1/\sqrt{\mathcal{N}})$.

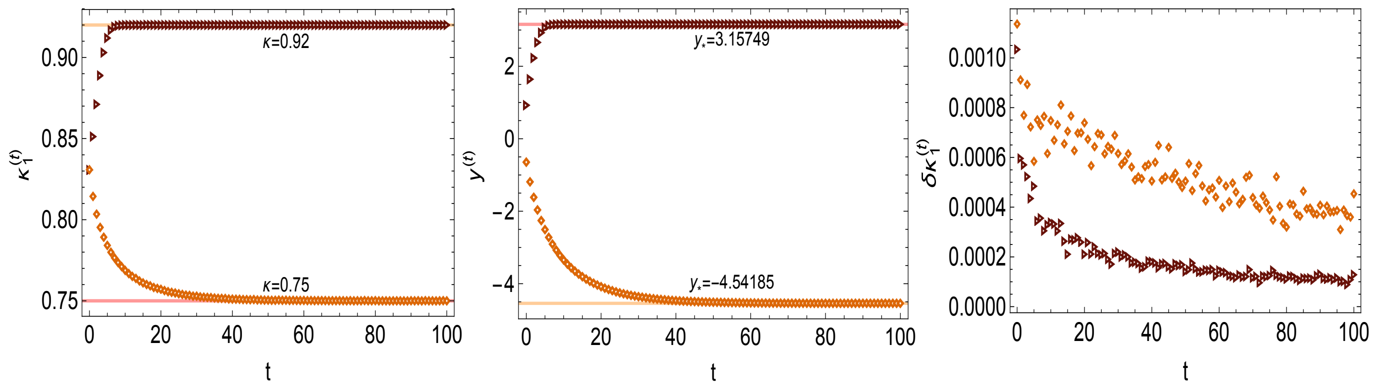


FIG. 1. Behavior of $\kappa_1^{(t)}$, $y^{(t)}$, and the standard deviation $\delta\kappa_1^{(t)}$ as a function of the iteration label $t$ in the Newton's method (see eq. (23)) for $k = 0.92$ (brown symbols) and $k = 0.75$ (orange symbols). These results are obtained by applying the weighted population dynamics algorithm to solve the system of self-consistency equations yielding the conditioned spectral density of ER random graphs with $c = 5$ and nonzero matrix elements, distributed according to $P_J(J) = (1//\sqrt{2\pi/c})e^{-cJ^2/2}$ (see the main text). For these plots we have used a population size which is increased linearly with each iteration step starting from $\mathcal{N} = 10^6$ up to $\mathcal{N} = 10^7$. The results are averaged over 100 runs of the population dynamics algorithm.
